# Supplementary material for: Focusing Knowledge-based Graph Argument Mining via Topic Modeling
Source: arXiv:2102.02086 source file (2021-02-03)
Supplement: Supplementary file 1 [file appendix.tex]

\section{Technical Appendix}

\begin{figure}[h]
    \centering
    \includegraphics[width=\columnwidth]{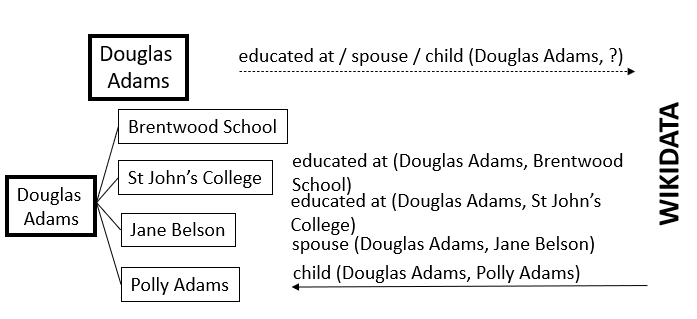}
    \caption{Improved expansion of the node "Douglas Adams" via one SPARQL query (dashed arrow) per entity.}
    \label{gfx:sparql_new}
\end{figure}
